# Supplementary material for: A hard-sphere quasicrystal stabilized by configurational entropy
Source: arXiv:2306.03549 ancillary file (2023-06-06)
Supplement: Supplementary file 1 [file SI.pdf]

# A hard-sphere quasicrystal stabilized by configurational entropy – Supplementary Information

Etienne Fayen[1], Laura Filion[2], Giuseppe Foffi[1], and Frank Smallenburg[1]
[1] *Université Paris-Saclay, CNRS, Laboratoire de Physique des Solides, 91405 Orsay, France*
[2] *Soft Condensed Matter, Debye Institute of Nanomaterials Science, Utrecht University, Utrecht, Netherlands*

## INFLATION

The quasicrystal configurations we use for our free-energy calculations are generated using an inflation procedure [1–3]. This procedure starts from a small seed tiling, and then iteratively replaces vertices in the tiling by dodecagonal wheels consisting of squares and triangles. Each wheel can in principle be placed in two orientations, and different choices of wheel orientations lead to different quasicrystal realizations, potentially with different symmetries. Here, we use three approaches. First, we produce deterministic quasicrystals with dodecagonal symmetry via the Schlottmann inflation rule [2, 3]. Second, we generate deterministic quasicrystals with hexagonal symmetry via the simpler Stampfli inflation rule [1]. Third, applying the Stampfli inflation rule with randomly chosen wheel orientations results in a limited ensemble of random tiling realizations with 12-fold symmetry on average. Examples of these tilings are shown in Fig. 1.

When starting from a square seed with Stampfli or Schlottmann rules, the inflated borders of the initial square

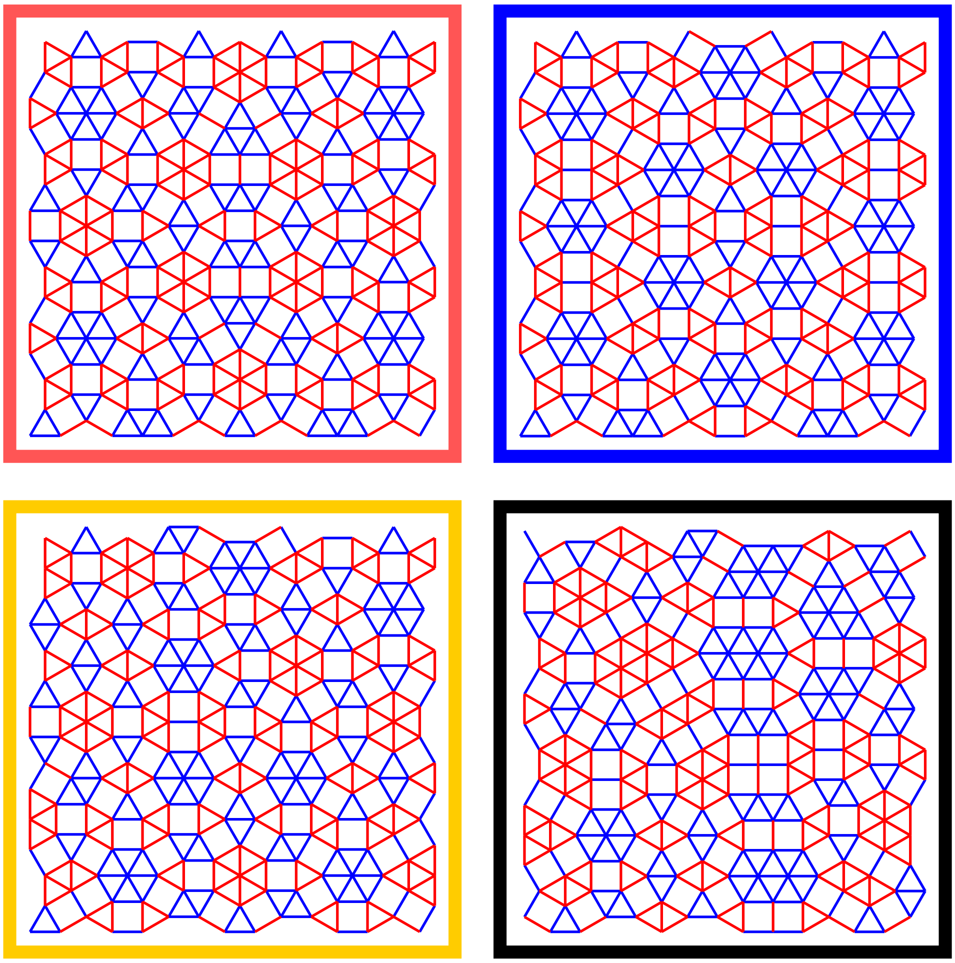

FIG. 1: Examples of the four types of tiling considered: Schlottmann tiling (top left), Stampfli tiling (top right), realization of a random Stampfli tiling (bottom left), and random tiling (bottom right).

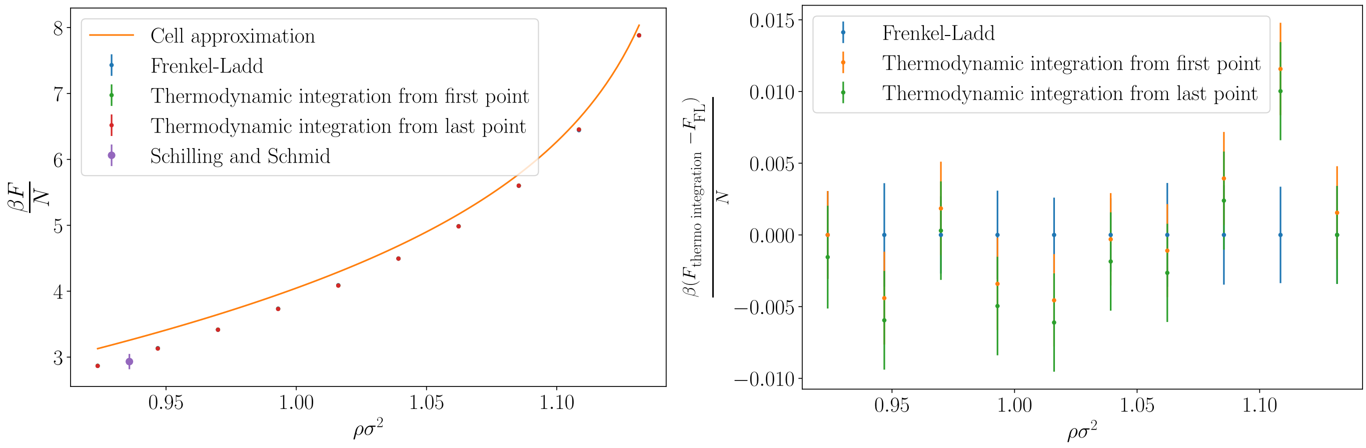


FIG. 2: (Left) Helmholtz free-energy of the hexagonal solid of hard disks computed from Frenkel-Ladd method (blue points), extrapolated from the first and last point with thermodynamic integration (red and green points) or reported by Schilling and Schmid in Ref. [6] purple point. The orange curve is corresponds to the cell approximation. (Right) Free-energy difference between the blue, red an green points that are almost indistinguishable on the left plot.

allow us to cut out square periodic approximants of the quasicrystal. We use this to generate our configurations. The number of particles in the tiling patch grows exponentially fast in the number of inflation iterations. Starting from a square seed, we used the configurations obtained after $n = 2, 3$ or 4 inflation steps, which corresponds to systems of $306, 4263$ and 59362 particles respectively. In addition, we generate Stamplfi tiling by applying 2 or 3 inflation steps to a sigma unit cell, which results into systems of 2284 and 31812 particles respectively. Since the orientation of the original sigma seed changes when the inflation rule is applied, our current implementation of the Schlottmann inflation fails in this case, so we only use the sigma seed to generate hexagonal Stampfli tilings. The exponential growth of the tilings with inflation iterations limits the number of available points for finite size scaling. However, the largest systems are large enough that we expect finite size corrections to be very small there. Other schemes exist, such as the Schlottmann half-step rule [4], that generates intermediate approximants, but its implementation is cumbersome, and we did not use it here. Likewise, seeds of intermediate size could be used, although, as described above, these can only be inflated with the tile-replacement approach, which we did not implement.

## ZIPPER MOVES

To generate random tiling configurations, we apply *zipper moves* to ideal configurations, following the approach introduced in Ref. [5]. A zipper move is a rearrangement of tiles around a closed loop that conserves the number of tiles of each type. Although to our knowledge, the ergodicity of the zippers has not been rigorously proven, numerical estimates of the square-triangle entropy based on zipper moves are consistent with the known exact value, suggesting that zipper moves indeed allow us to sample all configurations in the random tiling ensemble [5].

To obtain random tiling configurations for our free-energy calculations, we generate random configurations from ideal ones by applying 1000 zipper moves. Since the length of the zipper scales with the number of particles in the system [5], there is a priori no need to use more for larger systems. The generated configurations indeed look completely random and uncorrelated with the ideal starting point.

## FRENKEL-LADD VALIDATION

We use the pure hexagonal solid to validate our Frenkel-Ladd implementation. Figure 2-Left displays the free energy of hard disks for various densities computed with the Frenkel-Ladd method. The green and red points are obtained by thermodynamic integration from the first (or last) Frenkel-Ladd point. The points obtained from direct Frenkel-Ladd calculations or thermodynamic integration are almost indistinguishable in this representation. In Figure 2-Right, the free-energy difference between the thermodynamic integrations and direct Frenkel-Ladd simulations is shown. Error bars correspond to one standard error. The points are all consistent within 2 standard errors, which confirms that our implementation of the Frenkel-Ladd method yields accurate free-energy *differences*.

| | Schlottmann | Stampfli | Random Stampfli | Fully random (avg over 5 configurations) |
|---|---|---|---|---|
| Square seed 2 inflation steps | 1832 | 7021 | 9467 | 4513 |
| Square seed 3 inflation steps | 1787 | 3118 | 7955 | 1142 |
| Square seed 4 inflation steps | 99 | 145 | 173 | 55 |
| Sigma seed 2 inflation steps | | 5591 | 11849 | 3446 |
| Sigma seed 3 inflation steps | | 324 | 271 | 293 |

TABLE I: Number of free-energy independent calculations for each configuration. Our implementation of the Schlottmann inflation method does not support starting from a sigma seed.

To validate the absolute value of the computed free-energies, we show on Figure 2-Left the free-energy obtained from the cell approximation (orange curve). At large densities, when the cell approximation becomes good, the curve converges to the value computed with the Frenkel-Ladd method. In addition, the purple point corresponds to the free-energy value reported in Schilling and Schmid [6] for a solid of 100 hard disks at pressure 10 $k_BT\sigma^{-2}$. The corresponding density is obtained from the simulated equation of state. The resulting value is compatible with our Frenkel-Ladd calculations within the error bars. The reported system is much smaller than the one we use, so finite size effects are also expected. These observations give us confidence that our implementation of the Frenkel-Ladd method is working correctly.

After computing the phase diagram we obtain that at $x_S = 0$, the monodisperse system of hard disks freezes at pressure $9.2\, k_BT\sigma^{-2}$ very close to the value reported in large-scale simulations [7–9], providing an additional sanity check on the methods. We note however, that pinpointing the melting transition of monodisperse hard disks is complicated by to the emergence of an intermediate hexatic phase between the solid and the crystal, which we do not explore in detail here.

## FREE-ENERGY STATISTICS

In order to reduce the statistical error on the entropy, we repeat the Frenkel-Ladd calculation a very large number of times, summarised in table I.

We check that the repeated measurements follow a Gaussian distribution, and use the standard deviation of the outcomes, divided by the square root of the number of repetitions (*i.e.* the statistical error on the mean) as our error bars.


[1] Stampfli, P. A dodecagonal quasi-periodic lattice in two dimensions. *Helv. Phys. Acta* **59**, 1260–1263 (1986).
[2] Hermisson, J., Richard, C. & Baake, M. A Guide to the Symmetry Structure of Quasiperiodic Tiling Classes. *J. Phys. I France* **7**, 1003–1018 (1997).
[3] Frettloeh, D. A fractal fundamental domain with 12-fold symmetry. *Symmetry Cult. Sci* **22**, 237–246 (2011).
[4] Zeng, X. & Ungar, G. Inflation rules of square-triangle tilings: From approximants to dodecagonal liquid quasicrystals. *Philos. Mag.* **86**, 1093–1103 (2006).
[5] Oxborrow, M. & Henley, C. L. Random square-triangle tilings: A model for twelvefold-symmetric quasicrystals. *Phys. Rev. B* **48**, 6966–6998 (1993).
[6] Schilling, T. & Schmid, F. Computing absolute free energies of disordered structures by molecular simulation. *J. Chem. Phys.* **131**, 231102 (2009).
[7] Mak, C. H. Large-scale simulations of the two-dimensional melting of hard disks. *Phys. Rev. E* **73**, 065104 (2006).
[8] Bernard, E. P. & Krauth, W. Two-step melting in two dimensions: first-order liquid-hexatic transition. *Phys. Rev. Lett.* **107**, 155704 (2011).
[9] Engel, M. *et al.* Hard-disk equation of state: First-order liquid-hexatic transition in two dimensions with three simulation methods. *Phys. Rev. E* **87**, 042134 (2013).
